# Supplementary material for: Aspects of Gravitational Collapse and the formation of Spacetime Singularities
Source: arXiv:1709.01512 source file (2017-09-05)
Supplement: Supplementary file 1 [file appendix1.tex]

%*******************************************************************************
%****************************** Appendix *********************************
%*******************************************************************************
\chapter{Extending calculation to larger systems}\label{appendix1}

Using the ideas of Bloch's theorem, the numerical calculations for a finite system can be extended to a larger system (called a supercell) containing identical copies of unit cells (UC), each of size $30 \times 30$ for our case. Such a method is commonly known as `repeated zone scheme' (RZS) \cite{PhysRevB.66.214502}. Here, we extend our calculation on a supercell containing $k \times k$ UC. These RZS calculations are numerically inexpensive compared to the BdG calculations on corresponding larger system and are believed to produce correct results at least for low disorder strengths when impurity-impurity correlations are weak.

We used RZS to generate a denser spectrum in the calculation of DOS and FT-LDOS by considering a supercell containing $12 \times 12$ UC.
Besides, obtaining the $q_y \rightarrow 0$ limit of $\Lambda_{xx}$ is tricky from simulations on a finite system for calculation of the superfluid stiffness. This is because of the limited $q_y$ values available on a $30 \times 30$ system from which the actual extrapolation ($q_y \rightarrow 0$) is to be made. Unlike the sSC case, where the $\Lambda_{xx}(q_y \rightarrow 0)\approx a_0+a_2 q_y^2$ ($a_0$ and $a_2$ being constants), $\Lambda_{xx}(q_y)$ shows a sub-linear behavior for a wide range of $q_y$ (not necessarily small). It is thus essential to obtain data on larger systems using RZS for an appropriate $q_y \rightarrow 0$ extrapolation. A significant numerical demand still limits $k \sim 2$ to $3$. We finally used a polynomial fit: $\Lambda^{\rm RZS}_{xx}(q_y)=\sum_p a_p q^p_y$ for $p$ up to $3$ for the final extrapolation. Fortunately, we found both in the GIMT and IMT methods that the $a_0$ is not sensitive to $p$ for the moderate to large $V$.
